# Supplementary material for: BO Ceti: Dwarf Nova Showing Both IW And and SU UMa-Type Features
Source: arXiv:2106.15028 ancillary file (2021-06-28)
Supplement: Supplementary file 1 [file sibo.pdf]

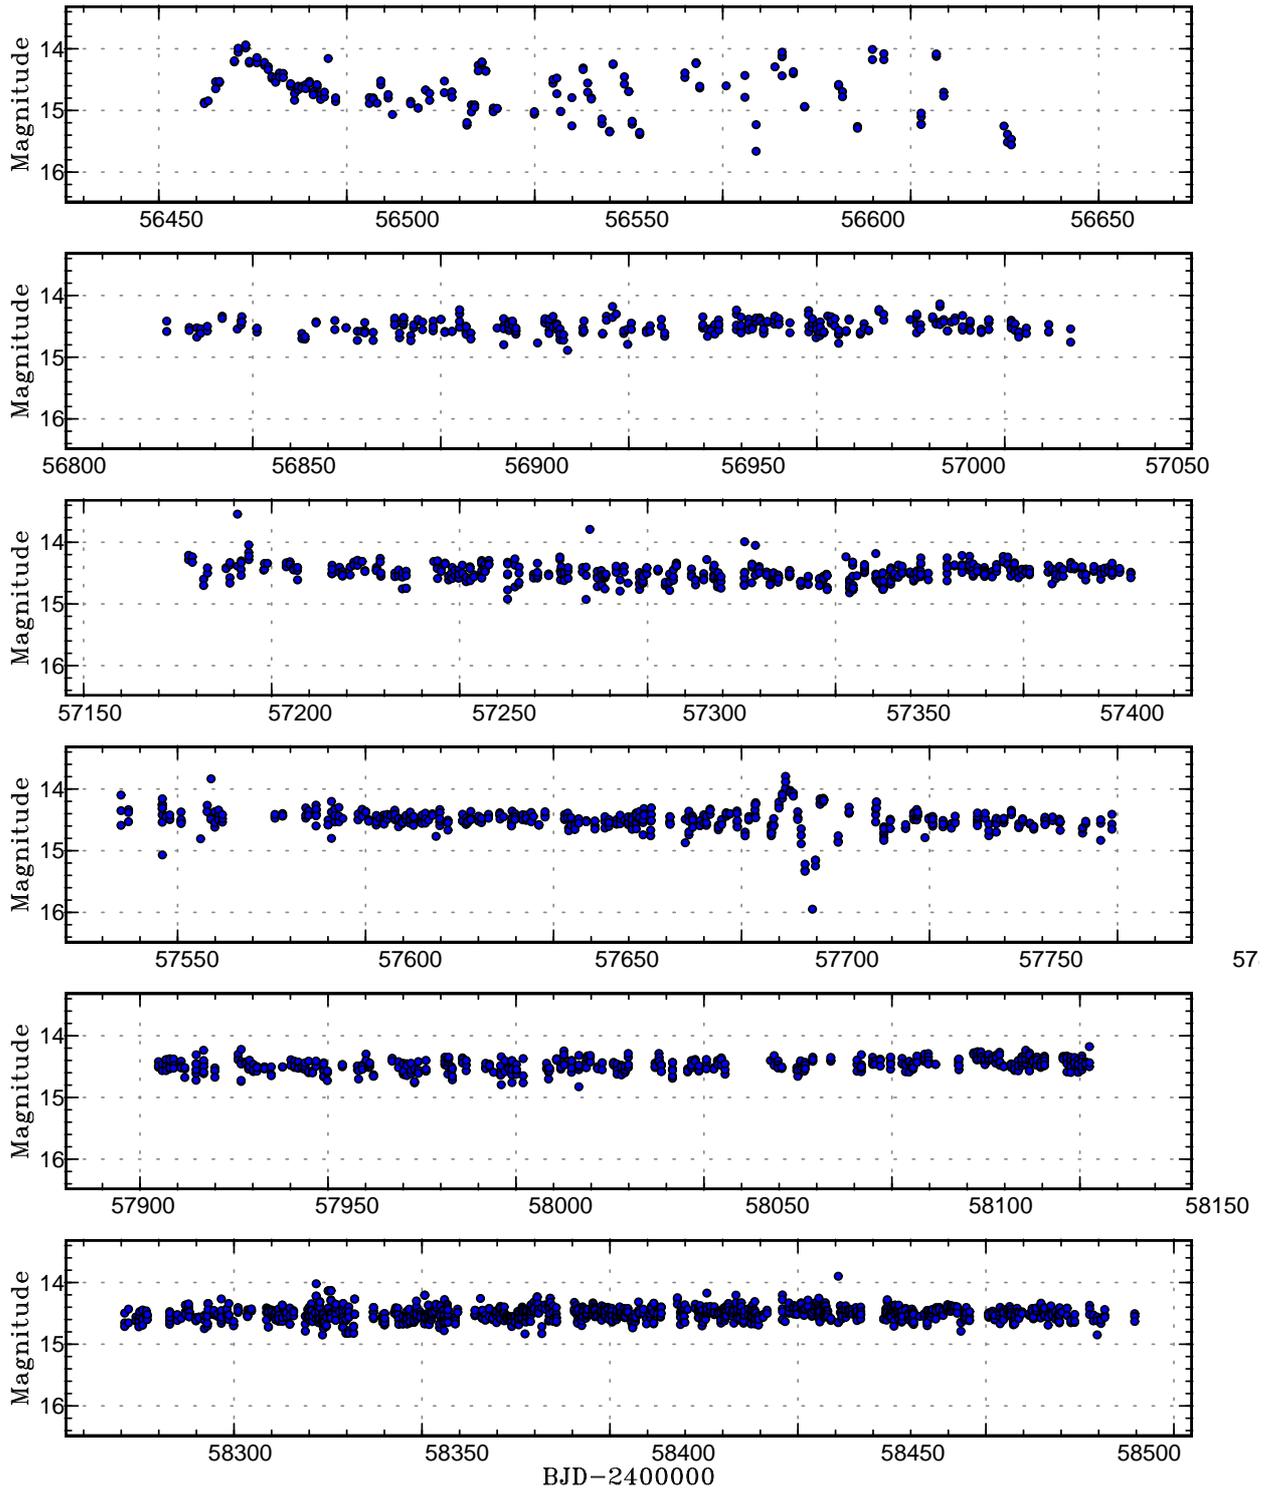

57

**E-figure 1.** Light curve of BO Cet between 2013 June and 2019 February based on ASAS-SN observations. The object mostly stayed in NL state (or standstill), but showed dwarf nova states in late 2013 (first panel) and 2017 November to December (fourth panel).

**E-table 1.** Superhump maxima of BO Cet (2020)

| $E$ | max*       | error  | $O - C^\dagger$ | $N^\ddagger$ |
|-----|------------|--------|-----------------|--------------|
| 0   | 59151.6746 | 0.0029 | -0.0294         | 30           |
| 1   | 59151.8298 | 0.0026 | -0.0249         | 25           |
| 6   | 59152.6083 | 0.0019 | -0.0001         | 30           |
| 13  | 59153.6811 | 0.0017 | 0.0175          | 27           |
| 14  | 59153.8265 | 0.0016 | 0.0123          | 29           |
| 26  | 59155.6447 | 0.0021 | 0.0217          | 35           |
| 27  | 59155.7920 | 0.0026 | 0.0182          | 25           |
| 33  | 59156.6897 | 0.0031 | 0.0116          | 22           |
| 34  | 59156.8318 | 0.0049 | 0.0029          | 29           |
| 39  | 59157.5769 | 0.0044 | -0.0056         | 25           |
| 40  | 59157.7335 | 0.0011 | 0.0002          | 21           |
| 41  | 59157.8758 | 0.0076 | -0.0082         | 18           |
| 43  | 59158.1895 | 0.0005 | 0.0041          | 433          |
| 46  | 59158.6445 | 0.0024 | 0.0068          | 35           |
| 47  | 59158.7863 | 0.0028 | -0.0021         | 25           |
| 49  | 59159.1018 | 0.0028 | 0.0119          | 98           |
| 51  | 59159.3924 | 0.0013 | 0.0010          | 77           |
| 52  | 59159.5283 | 0.0015 | -0.0138         | 68           |
| 53  | 59159.6806 | 0.0025 | -0.0122         | 22           |
| 78  | 59163.4554 | 0.0021 | -0.0057         | 81           |
| 79  | 59163.6179 | 0.0034 | 0.0061          | 54           |
| 86  | 59164.6615 | 0.0042 | -0.0055         | 28           |
| 86  | 59164.6612 | 0.0042 | -0.0058         | 27           |
| 89  | 59165.1182 | 0.0008 | -0.0010         | 766          |

\*BJD-2400000.

 $^\dagger$ Against max = 2459151.7040 + 0.150732E. $^\ddagger$ Number of points used to determine the maximum.

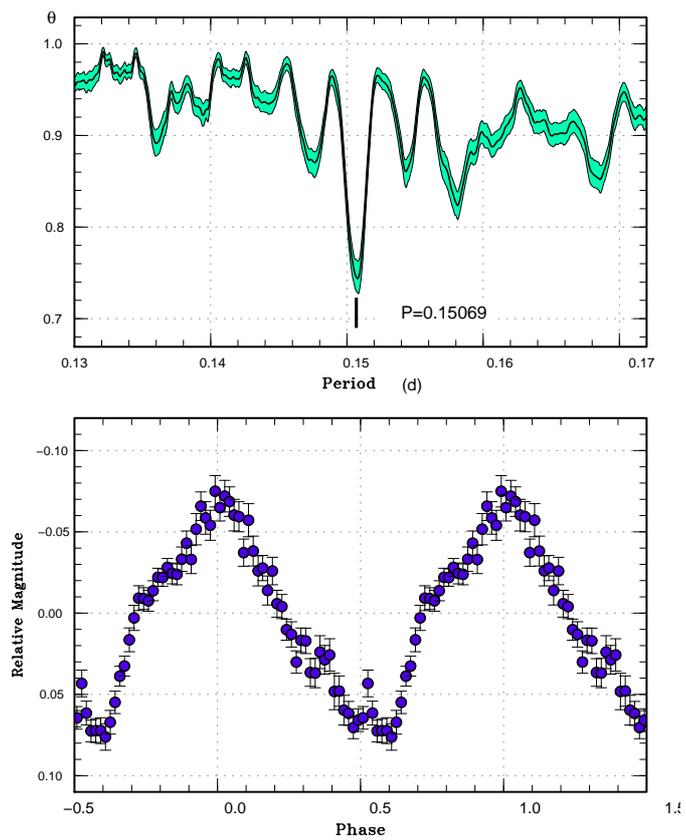

**E-figure 2.** Superhump profile of BO Cet. (Upper): PDM analysis. (Lower): Phase-averaged profile.
